# Supplementary material for: Differentiable Surface Splatting for Point-based Geometry Processing
Source: arXiv:1906.04173 source file (2019-09-03)
Supplement: Supplementary file 1 [file 07-appendix.tex]

\documentclass[acmtog, dvipsnames]{acmart}
%\acmSubmissionID{201}

% TOG prefers author-name bib system with square brackets
\citestyle{acmauthoryear}
\setcitestyle{nosort}
\setcitestyle{square}

\usepackage{units}
\usepackage[justification=centering]{subcaption}
\usepackage{booktabs} % For formal tables
\usepackage[flushleft]{threeparttable}
\usepackage{bbding}  % checkmark
\usepackage{amssymb}
\usepackage{wrapfig}
\usepackage{makecell}
\usepackage{multirow}
\usepackage[]{paralist}

\usepackage{enumitem}
\usepackage{arydshln} % dashed table line
\usepackage{url}

\usepackage{tikz}
\usetikzlibrary{spy,calc,shapes,arrows,positioning}
\input{99-pre.tex}

\acmJournal{TOG}

% Copyright
%\setcopyright{none}
%\setcopyright{acmcopyright}
%\setcopyright{acmlicensed}
\setcopyright{rightsretained}
%\setcopyright{usgov}
%\setcopyright{usgovmixed}
%\setcopyright{cagov}
%\setcopyright{cagovmixed}

% DOI
%\acmDOI{10.475/123_4}

% ISBN
%\acmISBN{123-4567-24-567/08/06}

%Conference
\acmJournal{TOG}
\acmYear{2019}\acmVolume{38}\acmNumber{4}\acmArticle{230}\acmMonth{7} \acmDOI{10.1145/3355089.3356513}
\copyrightyear{2019}

\begin{document}
	
	\title{Supplemental: Differentiable Surface Splatting for Point-based Geometry Processing}
	\author{Wang Yifan}
	\affiliation{%
		\institution{ETH Zurich}
		\country{Switzerland}
		%	\streetaddress{P.O. Box 1212}
		%	\city{Dublin}
		%	\state{Ohio}
		%	\postcode{43017-6221}
	}
	%\authornote{Both authors contributed equally to this research.}
	%\email{trovato@corporation.com}
	%\orcid{1234-5678-9012}
	\author{Felice Serena}
	%\authornotemark[1]
	%\email{webmaster@marysville-ohio.com}
	\affiliation{%
		\institution{ETH Zurich}
		%	\streetaddress{P.O. Box 1212}
		%	\city{Dublin}
		%	\state{Ohio}
		%	\postcode{43017-6221}
		\country{Switzerland}
	}
	
	\author{Shihao Wu}
	\affiliation{%
		\institution{ETH Zurich}
		%	\streetaddress{1 Th{\o}rv{\"a}ld Circle}
		%	\city{Hekla}
		\country{Switzerland}
	}
	%\email{larst@affiliation.org}
	
	\author{Cengiz {\"O}ztireli}
	\affiliation{%
		\institution{Disney Research Zurich}
		%	\city{Rocquencourt}
		\country{Switzerland}
	}
	
	\author{Olga Sorkine-Hornung}
	\affiliation{%
		\institution{ETH Zurich}
		%	\streetaddress{Rono-Hills}
		%	\city{Doimukh}
		%	\state{Arunachal Pradesh}
		\country{Switzerland}
	}
	%\author{Author 0}
	% \affiliation{%
	%   \institution{Affiliation 0}
	%    \city{City 0}
	%    \country{Country 0}
	% }
	% \email{author0@affiliation0.com}
	%
	%\author{Author 1}
	% \affiliation{%
	%   \institution{Affiliation 0}
	%    \city{City 0}
	%    \country{Country 0}
	% }
	% \email{author1@affiliation0.com}
	% 
	%\author{Author 2}
	% \affiliation{%
	%   \institution{Affiliation 0}
	%    \city{City 0}
	%    \country{Country 0}
	% }
	% \email{author2@affiliation1.com}
	% 
	%\author{Author 3}
	%\affiliation{%
	%   \institution{Affiliation 0}
	%    \city{City 0}
	%    \country{Country 0}
	% }
	% \email{author3@affiliation0.com}
	% 
	%\author{Author 4}
	%\affiliation{%
	%   \institution{Affiliation 0}
	%    \city{City 0}
	%    \country{Country 0}
	% }
	% \email{author4@affiliation0.com}
	
%	\begin{abstract}
%		\input{00-abstract}
%	\end{abstract}
	%\keywords{ACM proceedings, \LaTeX, text tagging}

	\begin{CCSXML}
		<ccs2012>
		<concept>
		<concept_id>10010147.10010371.10010396.10010400</concept_id>
		<concept_desc>Computing methodologies~Point-based models</concept_desc>
		<concept_significance>500</concept_significance>
		</concept>
		<concept>
		<concept_id>10010147.10010178.10010224</concept_id>
		<concept_desc>Computing methodologies~Computer vision</concept_desc>
		<concept_significance>200</concept_significance>
		</concept>
		<concept>
		<concept_id>10010147.10010257</concept_id>
		<concept_desc>Computing methodologies~Machine learning</concept_desc>
		<concept_significance>400</concept_significance>
		</concept>
		<concept>
		<concept_id>10010147.10010371.10010372</concept_id>
		<concept_desc>Computing methodologies~Rendering</concept_desc>
		<concept_significance>300</concept_significance>
		</concept>
		</ccs2012>
	\end{CCSXML}
	
	\ccsdesc[500]{Computing methodologies~Point-based models}
	\ccsdesc[200]{Computing methodologies~Computer vision}
	\ccsdesc[400]{Computing methodologies~Machine learning}
	\ccsdesc[300]{Computing methodologies~Rendering}
	
	\maketitle
	
%	\bibliographystyle{ACM-Reference-Format}
%	\bibliography{bibliography}
%	\pagebreak
	\appendix
	\input{appendix-content}

\bibliographystyle{ACM-Reference-Format}
\bibliography{bibliography}
\end{document}
